# Supplementary material for: Assessing the robustness of parsimonious predictions for gene neighborhoods from reconciled phylogenies
Source: arXiv:1503.05292 source file (2015-03-19)
Supplement: Supplementary file 1 [file appendix_isbra.tex]

\section*{Appendix for the reviewers}
%\vspace*{-10mm}%\begin{figure}[htbp]
\paragraph{The \DeCo{} DP algorithm.}~

\smallskip
\parindent=0cm
{\scriptsize
    \textbf{1}. If $e(g_1) = {\Extant}$ and $e(g_2) = {\Extant}$:\\
    $c_1(g_1, g_2) = 0$  if $g_1g_2$ is an extant adjacency and $\infty$ {otherwise}

    $c_0(g_1, g_2) = 0$  if $g_1g_2$ is not an extant adjacency and $\infty$ {otherwise}

    \textbf{2.} If $e(g_1) = {\GLos}$ and $e(g_2) \in \{{\Extant}, {\Spec}, {\GDup}\}$:
    $
    c_1(g_1, g_2) = c_0(g_1, g_2) = 0
    $
    
    \textbf{3.} If $e(g_1) \in \{{\Extant}, {\Spec}, {\GDup}\}$ and $e(g_2) = {\GLos}$:
    $
    c_1(g_1, g_2) = c_0(g_1, g_2) = 0
    $

    \textbf{4.} If $e(g_1) = {\GLos}$ and $e(g_2) = {\GLos}$:
    $
    c_1(g_1, g_2) = c_0(g_1, g_2) = 0
    $

    \textbf{5.} If $e(g_1) \in \{{\Extant}, {\Spec}\}$ and $e(g_2) = {\GDup}$:\\
    $
    c_1(g_1, g_2) =  \min
    \begin{cases}
      c_1(g_1,\cb{g_2}) + c_0(g_1,\ca{g_2}), c_0(g_1,\cb{g_2}) + c_1(g_1,\ca{g_2}), \\
      c_1(g_1,\cb{g_2}) + c_1(g_1,\ca{g_2}) + {\AGain},
      c_0(g_1,\cb{g_2}) + c_0(g_1,\ca{g_2}) + {\ABreak}% \\
    \end{cases}
    $
    \\
    $
    c_0(g_1, g_2) =  \min
    \begin{cases}
      c_0(g_1,\cb{g_2}) + c_0(g_1,\ca{g_2}),
      c_0(g_1,\cb{g_2}) + c_1(g_1,\ca{g_2}) + {\AGain}, \\
      c_1(g_1,\cb{g_2}) + c_0(g_1,\ca{g_2}) + {\AGain}, 
      c_1(g_1,\cb{g_2}) + c_1(g_1,\ca{g_2}) + 2{\AGain}% \\
    \end{cases}
    $

    \textbf{6.} If $e(g_1) = {\GDup}$ and $e(g_2) \in \{{\Extant}, {\Spec}\}$:\\
    $
    c_1(g_1, g_2) =  \min
    \begin{cases}
      c_1(\ca{g_1},g_2) + c_0(\cb{g_1},g_2),
      c_0(\ca{g_1},g_2) + c_1(\cb{g_1},g_2), \\
      c_1(\ca{g_1},g_2) + c_1(\cb{g_1},g_2) + {\AGain}, 
      c_0(\ca{g_1},g_2) + c_0(\cb{g_1},g_2) + {\ABreak}% \\
    \end{cases}
    $
    \\
    $
    c_0(g_1, g_2) =  \min
    \begin{cases}
      c_0(\ca{g_1},g_2) + c_0(\cb{g_1},g_2),
      c_0(\ca{g_1},g_2) + c_1(\cb{g_1},g_2) + {\AGain}, \\
      c_1(\ca{g_1},g_2) + c_0(\cb{g_1},g_2) + {\AGain}, 
      c_1(\ca{g_1},g_2) + c_1(\cb{g_1},g_2) + 2{\AGain}% \\
    \end{cases}
    $

    \textbf{7.} If $e(g_1) = {\Spec}$ and $e(g_2) = {\Spec}$:\\
    $
    c_1(g_1, g_2) =  \min
    \begin{cases}
      c_1(\ca{g_1},\cb{g_2}) + c_1(\cb{g_1},\ca{g_2}), 
      c_1(\ca{g_1},\cb{g_2}) + c_0(\cb{g_1},\ca{g_2}) + {\ABreak}, \\
      c_0(\ca{g_1},\cb{g_2}) + c_1(\cb{g_1},\ca{g_2}) + {\ABreak}, \\
      c_0(\ca{g_1},\cb{g_2}) + c_0(\cb{g_1},\ca{g_2}) + 2{\ABreak}, \\
      c_1(\ca{g_1},\ca{g_2}) + c_1(\cb{g_1},\cb{g_2}), 
      c_1(\ca{g_1},\ca{g_2}) + c_0(\cb{g_1},\cb{g_2}) + {\ABreak}, \\
      c_0(\ca{g_1},\ca{g_2}) + c_1(\cb{g_1},\cb{g_2}) + {\ABreak}, 
      c_0(\ca{g_1},\ca{g_2}) + c_0(\cb{g_1},\cb{g_2}) + 2{\ABreak}% \\
    \end{cases}
    $\\
    $
    c_0(g_1, g_2) =  \min
    \begin{cases}
      c_0(\ca{g_1},\cb{g_2}) + c_0(\cb{g_1},\ca{g_2}), 
      c_1(\ca{g_1},\cb{g_2}) + c_0(\cb{g_1},\ca{g_2}) + {\AGain}, \\
      c_0(\ca{g_1},\cb{g_2}) + c_1(\cb{g_1},\ca{g_2}) + {\AGain},
      c_1(\ca{g_1},\cb{g_2}) + c_1(\cb{g_1},\ca{g_2}) + 2{\AGain}, \\
      c_0(\ca{g_1},\ca{g_2}) + c_0(\cb{g_1},\cb{g_2}), 
      c_1(\ca{g_1},\ca{g_2}) + c_0(\cb{g_1},\cb{g_2}) + {\AGain}, \\
      c_0(\ca{g_1},\ca{g_2}) + c_1(\cb{g_1},\cb{g_2}) + {\AGain}, 
      c_1(\ca{g_1},\ca{g_2}) + c_1(\cb{g_1},\cb{g_2}) + 2{\AGain}%, \\
    \end{cases}
    $

    \textbf{8.} If $e(g_1) = {\GDup}$ and $e(g_2) = {\GDup}$:\\ 
    $
    c_1(g_1, g_2) =  \min
    \begin{cases}
      c_1(\ca{g_1},g_2) + c_0(\cb{g_1},g_2),
      c_0(\ca{g_1},g_2) + c_1(\cb{g_1},g_2), \\
      c_1(\ca{g_1},g_2) + c_1(\cb{g_1},g_2) + {\AGain},
      c_0(\ca{g_1},g_2) + c_0(\cb{g_1},g_2) + {\ABreak}, \\
      c_1(g_1,\ca{g_2}) + c_0(g_1,\cb{g_2}), 
      c_0(g_1,\ca{g_2}) + c_1(g_1,\cb{g_2}), \\
      c_1(g_1,\ca{g_2}) + c_1(g_1,\cb{g_2}) + {\AGain}, 
      c_0(g_1,\ca{g_2}) + c_0(g_1,\cb{g_2}) + {\ABreak}, \\
      c_1(\ca{g_1},\ca{g_2}) + c_1(\cb{g_1},\cb{g_2}) + c_0(\ca{g_1},\cb{g_2}) + c_0(\cb{g_1},\ca{g_2}), \\
      c_1(\ca{g_1},\ca{g_2}) + c_1(\cb{g_1},\cb{g_2}) + c_0(\ca{g_1},\cb{g_2}) + c_1(\cb{g_1},\ca{g_2}) + {\AGain}, \\
      c_1(\ca{g_1},\ca{g_2}) + c_1(\cb{g_1},\cb{g_2}) + c_1(\ca{g_1},\cb{g_2}) + c_0(\cb{g_1},\ca{g_2}) + {\AGain}, \\
      c_1(\ca{g_1},\ca{g_2}) + c_1(\cb{g_1},\cb{g_2}) + c_1(\ca{g_1},\cb{g_2}) + c_1(\cb{g_1},\ca{g_2}) + 2{\AGain}, \\
      c_1(\ca{g_1},\ca{g_2}) + c_0(\cb{g_1},\cb{g_2}) + c_0(\ca{g_1},\cb{g_2}) + c_0(\cb{g_1},\ca{g_2}) + {\ABreak}, \\
      c_1(\ca{g_1},\ca{g_2}) + c_0(\cb{g_1},\cb{g_2}) + c_0(\ca{g_1},\cb{g_2}) + c_1(\cb{g_1},\ca{g_2}) + {\AGain} + {\ABreak}, \\
      c_1(\ca{g_1},\ca{g_2}) + c_0(\cb{g_1},\cb{g_2}) + c_1(\ca{g_1},\cb{g_2}) + c_0(\cb{g_1},\ca{g_2}) + {\AGain} + {\ABreak}, \\
      c_0(\ca{g_1},\ca{g_2}) + c_1(\cb{g_1},\cb{g_2}) + c_0(\ca{g_1},\cb{g_2}) + c_0(\cb{g_1},\ca{g_2}) + {\ABreak}, \\
      c_0(\ca{g_1},\ca{g_2}) + c_1(\cb{g_1},\cb{g_2}) + c_0(\ca{g_1},\cb{g_2}) + c_1(\cb{g_1},\ca{g_2}) + {\AGain} + {\ABreak}, \\
      c_0(\ca{g_1},\ca{g_2}) + c_1(\cb{g_1},\cb{g_2}) + c_1(\ca{g_1},\cb{g_2}) + c_0(\cb{g_1},\ca{g_2}) + {\AGain} + {\ABreak}, \\
      c_0(\ca{g_1},\ca{g_2}) + c_0(\cb{g_1},\cb{g_2}) + c_1(\ca{g_1},\cb{g_2}) + c_1(\cb{g_1},\ca{g_2}), \\
      c_0(\ca{g_1},\ca{g_2}) + c_1(\cb{g_1},\cb{g_2}) + c_1(\ca{g_1},\cb{g_2}) + c_1(\cb{g_1},\ca{g_2}) + {\AGain}, \\
      c_1(\ca{g_1},\ca{g_2}) + c_0(\cb{g_1},\cb{g_2}) + c_1(\ca{g_1},\cb{g_2}) + c_1(\cb{g_1},\ca{g_2}) + {\AGain}, \\
      c_0(\ca{g_1},\ca{g_2}) + c_0(\cb{g_1},\cb{g_2}) + c_1(\ca{g_1},\cb{g_2}) + c_0(\cb{g_1},\ca{g_2}) + {\ABreak}, \\
      c_0(\ca{g_1},\ca{g_2}) + c_0(\cb{g_1},\cb{g_2}) + c_0(\ca{g_1},\cb{g_2}) + c_1(\cb{g_1},\ca{g_2}) + {\ABreak}, \\
      c_0(\ca{g_1},\ca{g_2}) + c_0(\cb{g_1},\cb{g_2}) + c_0(\ca{g_1},\cb{g_2}) + c_0(\cb{g_1},\ca{g_2}) + 2{\ABreak}%, \\
    \end{cases}
    $\\
    $
    c_0(g_1, g_2) =  \min
    \begin{cases}
      c_0(\ca{g_1},g_2) + c_0(\cb{g_1},g_2), 
      c_0(\ca{g_1},g_2) + c_1(\cb{g_1},g_2) + {\AGain}, \\
      c_1(\ca{g_1},g_2) + c_0(\cb{g_1},g_2) + {\AGain},
      c_1(\ca{g_1},g_2) + c_1(\cb{g_1},g_2) + 2{\AGain}, \\
      c_0(g_1,\ca{g_2}) + c_0(g_1,\cb{g_2}), 
      c_0(g_1,\ca{g_2}) + c_1(g_1,\cb{g_2}) + {\AGain}, \\
      c_1(g_1,\ca{g_2}) + c_0(g_1,\cb{g_2}) + {\AGain},
      c_1(g_1,\ca{g_2}) + c_1(g_1,\cb{g_2}) + 2{\AGain}%, \\
    \end{cases}
    $

%    \vspace*{-2mm}
%    \caption{The \DeCo{} dynamic programming equations, adapted from~\cite{DBLP:journals/bioinformatics/BerardGBSDT12}.}
%  \label{fig:deco}
%\end{figure}
}

\vfill\pagebreak

\paragraph{Boltzmann/Ensembl approach.}
In \cite{DBLP:conf/wob/ChauvePZ14}, we showed how to extend the
\DeCo{} algorithm to an ensemble approach that allows one to explore the
whole solution space of adjacency forests. Let  ${\mathcal
  F}(G_1,G_2)$ be the set of all adjacency forests for $G_1$ and
$G_2$, including both optimal and sub-optimal ones.  The {\em
  partition function} associated to $G_1$ and $G_2$ is defined by
$$\PF(G_1,G_2)=\sum_{A\in {\mathcal F}(G_1,G_2)} e^{-\frac{S(A)}{kT}}$$
where $kT$ is an arbitrary constant.  
The partition function implicitly defines a {\em Boltzmann probability
  distribution} over ${\mathcal F}(G_1,G_2)$, where the probability of an
adjacency forest $A$ is defined by:
$$P(A)=\frac{e^{-\frac{S(A)}{kT}}}{\PF(G_1,G_2)}.$$ The Boltzmann
probability of an adjacency, or more generally of a feature that can
be observed in an adjacency forest, is then defined as the ratio of
the sum of the Boltzmann probabilities of the adjacency forests that
contain this feature. Such probabilities can be computed efficiently
using a variation of the dynamic programming algorithm of
\DeCo{}~\citep{DBLP:conf/wob/ChauvePZ14}.  The impact of $kT$ on the
Boltzmann probability can be described as follows: when $kT$ is small,
the Boltzmann distribution probability is skewed toward parsimonious
adjacency forests, while a high value of $kT$ tends toward a more
uniform probability distribution.
